# Supplementary material for: The 2024 Foundation Model Transparency Index
Source: arXiv:2407.12929 source file (2025-03-04)
Supplement: Supplementary file 1 [file app_succinct_disclosures.tex]

\hypertarget{succinct}{\section{Succinct disclosures}}
\label{app:succinct-disclosures}

By publishing transparency reports submitted by many major AI developers, we effectively centralize information about their practices.
In turn, this centralized information, which is also organized in accordance with the indicator structure of FMTI, functions as new resource for researching these practices.
Of the 100 transparency indicators, we identify a subset of 36 indicators with succinct disclosures.
The resulting 36 $\times$ 14 matrix of selected information across all developers, with some post-processing to increase clarity, is made available in \autoref{tab:succinct-disclosures}.

\tiny
\begin{longtblr}[
  caption = {\textbf{Developer Disclosures for 36 Indicators.}},
  label = {tab:succinct-disclosures},
]{
  colspec = {|Xcccccccccccccc|},
  rowhead = 1,
  hlines,
  row{even} = {gray9},
  row{1} = {olive9},
} 
    
& Adept & AI21 & Aleph Alpha & Amazon & Anthropic & BC/HF/SN & Google & IBM & Meta & Microsoft & Mistral & OpenAI & Stability & Writer \\
\hline        
\textbf{Data size} & 500 tok & 500 tok & 500 tok & 500 tok & 500 tok & 500 tok & 500 tok & 500 tok & 500 tok & 500 tok & 500 tok & 500 tok & 500 tok & 500 tok  \\ 
\end{longtblr}
\clearpage
% Revert to initial values
\eject
\pdfpagewidth=\originalwidth \pdfpageheight=\originalheight
\newgeometry{top=2cm, head=10pt, left=2cm, right=2cm,bottom=2cm}
